# Supplementary material for: Blending Reward Functions via Few Expert Demonstrations for Faithful and Accurate Knowledge-Grounded Dialogue Generation
Source: arXiv:2311.00953 source file (2023-11-02)
Supplement: Supplementary file 1 [file appendix.tex]

\section{Example Appendix}
\label{sec:appendix}

This is a section in the appendix.
